# Supplementary material for: Coupled Spin-Charge-Phonon Fluctuation in the All-In/All-Out Antiferromagnet Cd$_2$Os$_2$O$_7$
Source: arXiv:1911.12500 source file (2019-11-28)
Supplement: Supplementary file 1 [file cdoso-suppl.pdf]

# Supplemental Material

A. Koda,[1,2] H. Hirose,[3,*] M. Miyazaki,[1,†] H. Okabe,[1,2] M. Hiraishi,[1] I. Yamauchi,[1,‡]
K. M. Kojima,[1,2,§] I. Nagashima,[3] J. Yamaura,[3,¶] Z. Hiroi,[3] and R. Kadono[1,2,**]

[1]*Muon Science Laboratory and Condensed Matter Research Center, Institute of Materials Structure Science, High Energy Accelerator Research Organization (KEK), Tsukuba, Ibaraki 305-0801, Japan*
[2]*Department of Materials Structure Science, The Graduate University for Advanced Studies, Japan*
[3]*Institute for Solid State Physics, University of Tokyo, Kashiwa, Chiba 277-8581, Japan*

### $T_2$ anomaly in the AIAO phase of $Cd_2Os_2O_7$

As pointed out in the main text, the loss of $\mu$SR signal around $T_H$ is induced by the sharp increase of the longitudinal relaxation rate ($\lambda_\parallel$, $\lambda_\parallel^*$) with increasing fluctuation frequency $\nu$ towards the Larmor frequency $\omega$, known as "$T_1$ minimum" in NMR. In the case of the AIAO phase, $\lambda_\parallel$ and the corresponding transverse relaxation rate $\lambda_\perp$ can be approximated to yield [see Eqs. (7), (8) in the main text]

$$\lambda_\parallel = 1/T_1 \simeq \frac{2\omega_{\rm m}^2\nu}{\nu^2+\omega_{\rm m}^2}, \quad (1)$$

$$\lambda_\perp = 1/T_2 \simeq \frac{\lambda_\parallel}{2} + \lambda_{\rm m}, \quad (2)$$

where the $T_1$ minimum (i.e., the maximum in $\lambda_\parallel$) occurs when $\nu$ matches the Larmor frequency $\omega_{\rm m}$ determined by the internal field $B_{\rm m}$ at the muon site under a zero external field. [While $1/T_2$ refers only to the second term ($\lambda_{\rm m}$) in Eq. (2) in the NMR convention, we use the term defined as above.] Since $\lambda_\perp$ is also enhanced in accordance with $\lambda_\parallel$, it would exceed $\omega_{\rm m}/2\pi$ at certain temperature $T_H$ above which muon cannot maintain the coherent spin precession. The situation is illustrated in Fig. S1a, where one can observe that $\lambda_\parallel$ calculated assuming the temperature dependence for the fluctuation rate deduced from our $\mu$SR data, $\nu = 4.5 \times 10^7 \exp[-2436/T(\mathrm{K})]$ (MHz), exceeds $\omega_{\rm m}/2\pi$ around $T_H$.

In the case of $Cd_2Os_2O_7$, there are two channels of excitations that induce $\boldsymbol{\Delta B}_{\rm m}$, one is the conventional magnon/spin-wave excitation ($\nu \sim$THz, which is mainly determined by the exchange interaction), and another is the carrier-driven spin excitation ($\nu \sim$MHz-GHz, which would be relevant only for the narrow-gap semiconductors like $Cd_2Os_2O_7$). While the characteristic $\nu$ for the magnon/spin excitation is orders of magnitude higher than $\omega_{\rm m}$, that of the carrier-driven spin excitation comes close to $\omega_{\rm m}$ to cause sharp increase of $\lambda_\parallel$ around $T_H$. Needless to mention that such a resonant relaxation process is absent in neutron/X-ray as well as magnetic susceptibility measurements.

In order to examine the consistency of the $T_1$-minimum model with other experiments, we investigated the unpublished $^{17}$O-NMR data on single-crystalline $Cd_2Os_2O_7$ [1], and found that a similar loss of signals might have been observed near $T_N = 227$ K. More specifically, among the signals from six $^{17}$O nuclei of $OsO_6$ octahedron under an external field $\boldsymbol{B}_0 \parallel [100]$ axis, the signal from O(6) site (for which the hyperfine field $\boldsymbol{B}_{\rm m}$ was antiparallel with $\boldsymbol{B}_0$) disappeared at $\sim$220 K, while that from O(1) site

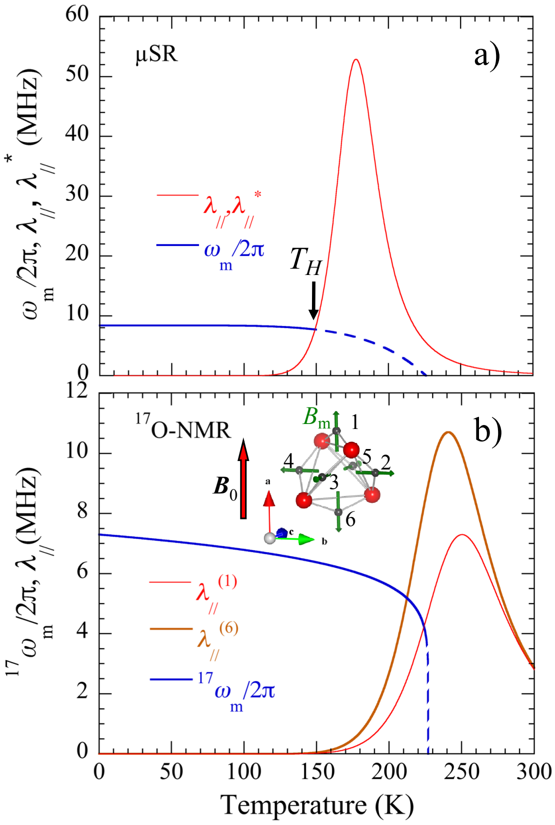


FIG. S1. (a) Longitudinal muon spin relaxation rate $\lambda_\parallel$ ($\lambda_\parallel^*$) versus emperature ($T$) calculated by the spin fluctuation rate $\nu(T)$ deduced from the present $\mu$SR experiment, which is plotted together with $\omega_{\rm m}/2\pi$. $\lambda_\parallel$ exceeds $\omega_{\rm m}/2\pi$ at $T_H \simeq 150$ K while it increases towards the peak (corresponding to the $T_1$ minimum). (b) Predicted $T$ dependence of $1/T_1 = \lambda_\parallel$ for O(1) and O(6) sites in $^{17}$O-NMR measurements. Inset shows the local atomic configuration consisting of four Os ions (red balls) at the corners of tetrahedron and nn oxygen atoms corresponding to O(1)-O(6).

was observed. In the abovementioned model, we have

$$\lambda_\parallel = 1/T_1 \simeq \frac{2({}^{17}\omega_{\rm m})^2\nu}{\nu^2 + (\gamma_I B_0 \pm {}^{17}\omega_{\rm m})^2}, \quad (3)$$

where $\gamma_I B_0 = 240$ MHz ($B_0 = 6.6147$ T), and ${}^{17}\omega_{\rm m} = 45.7$ MHz (at 20 K, $B_{\rm m} = 1.26$ T) with + and − corresponding to O(1) and O(6), respectively. Assuming the common temperature dependence for $\nu$, $\lambda_\parallel$ calculated by Eq. (3) for the each O site is shown in Fig. S1b. It is observed that $\lambda_\parallel$ becomes comparable with ${}^{17}\omega_{\rm m}/2\pi$ at 210 K and 220 K for the respective sites, predicting that the signal from O(6) site will be lost at lower temperatures than that from O(1), which is qualitatively in line with the preliminary experimental result. While the fact that the O(6) signal showing lower frequency than the O(1) signal indicates that the loss is not due to experimental artifacts (e.g., temperature fluctuation, etc.), the closeness of the relevant temperature to $T_N$ may call for more precise measurements. In any case, it should be stressed that the absence of such effect around $T_H \simeq 150$ K for ${}^{17}$O-NMR is perfectly in line with the present interpretation of our $\mu$SR result.

It is tempting to speculate that the anomalous loss of resonance signal often encountered in the NMR studies of magnetic compounds may have the similar cause, where the frequency range of spin fluctuation as well as experimental parameters accidentally satisfy the condition for the $T_1$ minimum.

* Present address: National Institute for Materials Science, Tsukuba, Ibaraki 305-0003, Japan

† Present address: Muroran Institute of Technology, Muroran, Hokkaido 050-8585, Japan

‡ Present address: Department of Physics, Graduate School of Science and Engineering, Saga University, Saga 840-8502, Japan

§ Present address: Centre for Molecular and Materials Science, TRIUMF, Vancouver, BC V6T2A3, Canada

¶ Present address: Materials Research Center for Element Strategy, Tokyo Institute of Technology, Yokohama, Kanagawa 226-8503, Japan

** e-mail: ryosuke.kadono@kek.jp

[1] I. Yamauchi, M. Takigawa, J. Yamaura, and Z. Hiroi, unpublished.
